# Supplementary material for: Transition from ferromagnetic to noncollinear to paramagnetic state with increasing Ru concentration in FeRu films
Source: arXiv:2407.17575 source file (2024-07-24)
Supplement: Supplementary file 1 [file Supplemental.pdf]

# Supplemental Material for:
# Transition from ferromagnetic to noncollinear to paramagnetic state with increasing Ru concentration in FeRu films

Juliana Lisik,[1,*] Manuel Rojas,[1,†] Spencer Myrtle,[1] Dominic H. Ryan,[2,‡] René Hübner,[3] Pavlo Omelchenko,[1] Claas Abert,[4] Amil Ducevic,[4] Dieter Suess,[4] Ivan Soldatov,[5] Rudolf Schaefer,[5] Johannes Seyd,[6] Manfred Albrecht,[6] and Erol Girt[1,§]

[1]*Simon Fraser University, 8888 University Drive, Burnaby, British Columbia V5A 1S6, Canada*
[2]*Physics Department and Centre for the Physics of Materials, McGill University, 3600 University Street, Montreal, Quebec, H3A 2T8, Canada*
[3]*Institute of Ion Beam Physics and Materials Research, Helmholtz-Zentrum Dresden-Rossendorf, Bautzner Landstraße 400, 01328 Dresden, Germany*
[4]*Physics of Functional Materials, Faculty of Physics, University of Vienna, Kolingasse 14–16, 1090 Vienna, Austria*
[5]*Leibniz-Institut für Festkörper- und Werkstoffforschung Dresden, Germany*
[6]*Institute of Physics, University of Augsburg, 86135 Augsburg, Germany*
(Dated: June 3, 2024)

## I. TRANSMISSION ELECTRON MICROSCOPY FOR Ta|Ru|Fe|Ru FILM

To analyze the diffusion of Ru into the pure Fe film, cross-sectional TEM characterization was performed on Ta|Ru|Fe(100)|Ru. The bright-field TEM image in Fig. S1(a) shows that our films have columnar grain growth. Quantifying the EDXS signal in Fig. S1(b) from the whole Fe layer, a Ru content of 0.1 at. % was determined. This could either be due to the diffusion of Ru into the Fe layer during the sputtering process or due to the introduction of Ru into the Fe layer during the TEM lamella preparation process.

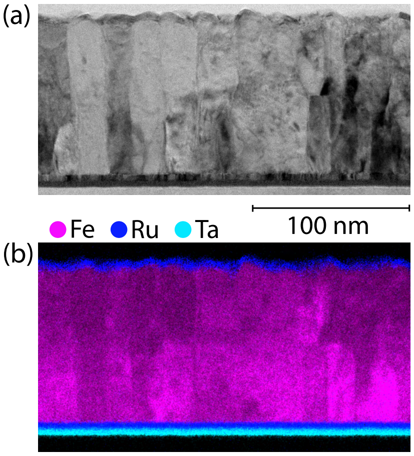


FIG. S1. (a) Bright-field TEM and (b) STEM-EDXS-based element distribution maps of Ta(3.5)|Ru(3.5)|Fe(100)|Ru(3.5).

* jbesler@sfu.ca
† mrojas@sfu.ca
‡ dhryan@physics.mcgill.ca
§ egirt@sfu.ca

## II. MICROMAGNETIC SIMULATIONS OF Fe FILM

Micromagnetic simulations of an 100 nm-thick Fe film of size 1 µm × 1 µm were performed. When a 0.05 T in-plane magnetic field is applied, the magnetization of the film fully saturates along the field direction with no magnetic domains and no out-of-plane magnetization component. The results presented in Fig. S2 represent the relaxed state of the film after the magnetic field is removed. Figure S2(a) is a top view of the magnetic moment distribution, and Fig. S2(b) is a top view of the projection of the magnetization along the field direction after the field is removed. The colour red represents a magnetic moment in the film that is fully aligned with the field direction, while the colour blue represents a magnetic moment that is pointing in the opposite direction of the previously-applied field. The average out-of-plane angle of the magnetization obtained from these simulations is $(6 \pm 10)^\circ$ from the film plane ($(84 \pm 10)^\circ$ from the film normal) in the absence of the external magnetic field.

## III. $M_r/M_s$ CALCULATIONS

We will consider films consisting of non-interacting magnetic grains with the easy axes of the magnetic grains randomly distributed in all three directions (x, y, and z). We will also neglect the demagnetization field in these calculations. If a large magnetic field is applied perpendicular to the film surface (in the z-direction) and then removed, the magnetic moments of the grains will be randomly distributed in a hemisphere above the film surface, as shown in Fig. S3(a). Assuming that each magnetic grain has the same magnetic moment, $m_s$, the $M_r/M_s$ ratio can be calculated as

$$\frac{M_r}{M_s} = \frac{m_z}{m_s} = \frac{m_s^3 \left(\int_0^{\pi/2} \sin\theta \cos\theta \; d\theta\right) \int_0^{2\pi} d\phi}{m_s^3 \left(\int_0^{\pi/2} \sin\theta \; d\theta\right) \int_0^{2\pi} d\phi} = \frac{1}{2}, \quad (1)$$

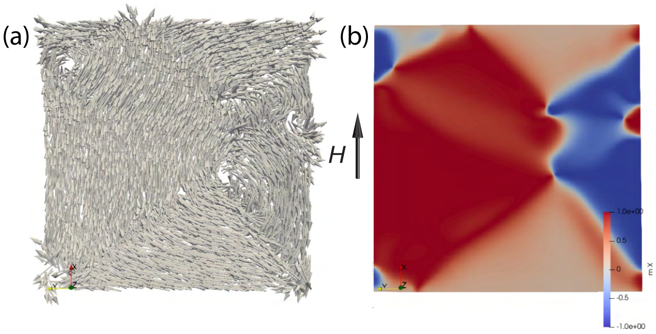


FIG. S2. Micromagnetic simulations of 100 nm-thick Fe film of size 1 µm × 1 µm after an external magnetic field of 0.05 T is applied in the plane and then removed. Top view of the film plane showing (a) the magnetic moment distribution and (b) the projection of the magnetization along the field direction. The colour key spans from magnetization completely opposite the field direction (blue) to magnetization completely along the field direction (red).

where $m_z$ is the average projection of $m_s$ in the magnetic field direction (z-direction) after the field is removed. The angles $\theta$ and $\phi$ are the spherical coordinates, labelled in Fig. S3(a).

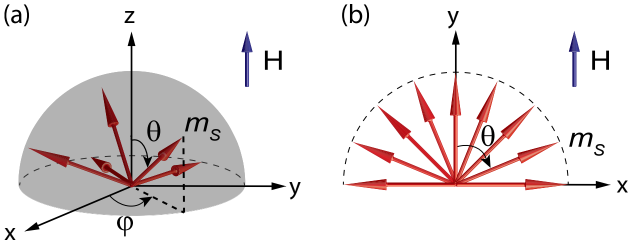


FIG. S3. Schematic of non-interacting magnetic moments $m_s$ that are randomly distributed in (a) a hemisphere and (b) a semicircle. This represents a simplified model of a ferromagnetic material consisting of non-interacting magnetic grains with randomly-oriented easy axes, where each grain has the same magnetic moment $m_s$.

Next, we will take into account the demagnetizing field, which is oriented in the plane of the film and can be very large in magnetic films with a high saturation magnetization. In Fe films, the demagnetizing field is $\mu_0 M_s = 2.15\,\mathrm{T}$, where $M_s = 1.711\,\mathrm{MA/m}$. If the demagnetizing field in a film is much larger than the anisotropy field of the magnetic grains, the magnetic moments of the grains will lie in the film plane but will be free to orient randomly within it. If a large in-plane magnetic field is applied in the y-direction and then removed, the magnetic moments of the grains will be randomly distributed in a semicircle in the xy-plane, as shown in Fig. S3(b). Assuming that each magnetic grain has the same magnetic moment, $m_s$, the $M_r/M_s$ ratio can be calculated as

$$\frac{M_r}{M_s} = \frac{m_y}{m_s} = \frac{m_s^2 \int_0^{\pi/2} \cos\theta \, d\theta}{m_s^2 \int_0^{\pi/2} d\theta} = \frac{2}{\pi} \approx 0.64, \qquad (2)$$

where $m_y$ is the average projection of $m_s$ in the magnetic field direction (y-direction) after the field is removed and $\theta$ is the angle between $m_s$ and the field direction.

## IV. LORENTZ TRANSMISSION ELECTRON MICROSCOPY VIDEO OF SWITCHING EVENTS IN $Fe_{92}Ru_8$ FILM

The magnetization reversal process of a Ta|Ru|$Fe_{92}Ru_8$(20)|Ru film was investigated by Lorentz transmission electron microscopy (LTEM). The sample was prepared by magnetron sputter deposition on a 30 nm-thick $Si_3N_4$ membrane. Magnetic fields are applied along the electron beam direction, which is typically perpendicular to the film plane. Thus, the sample was tilted by a tilt angle $\theta$ with respect to the film normal, yielding an in-plane magnetic field of $H_{\mathrm{IP}} = H_{\mathrm{appl}} \sin\theta$ and an out-of-plane magnetic field of $H_{\mathrm{OOP}} = H_{\mathrm{appl}} \cos\theta$.

Prior to acquiring images, the sample was tilted at $\theta = -40°$ with respect to the film normal in an applied magnetic field of about 2 T to align the in-plane magnetization of the sample toward the negative direction. $H_{\mathrm{appl}}$ was then increased to zero in order to bring the in-plane magnetization to the negative remanence point. Images were then acquired at room temperature with the sample tilted at $\theta = +40°$, beginning at the negative remanence point and increasing $H_{\mathrm{appl}}$ in steps.

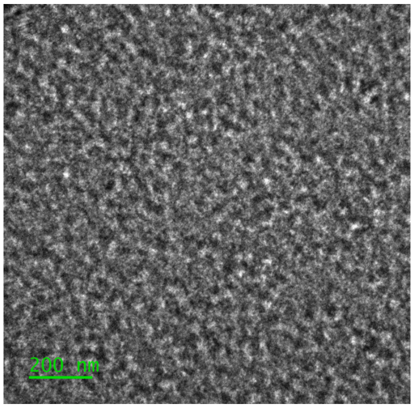


Video S1. Video acquired via Lorentz transmission electron microscopy of a Ta|Ru|$Fe_{92}Ru_8$(20)|Ru film as an external magnetic field is applied. For the first 5 s, the field is stable at 96 mT, and from 5 to 14 s, it is increased to 112 mT in 12 steps. From 15 s onwards, the field is stable at 112 mT.

Individual reversal events can be observed in Video S1, which was recorded via LTEM of a sample area as an external magnetic field was increased from 96 to 112 mT.
